# Supplementary material for: Electroluminescence and Energy Transfer Mediated by Hyperbolic Polaritons
Source: arXiv:2310.08351 source file (2024-12-02)

**a**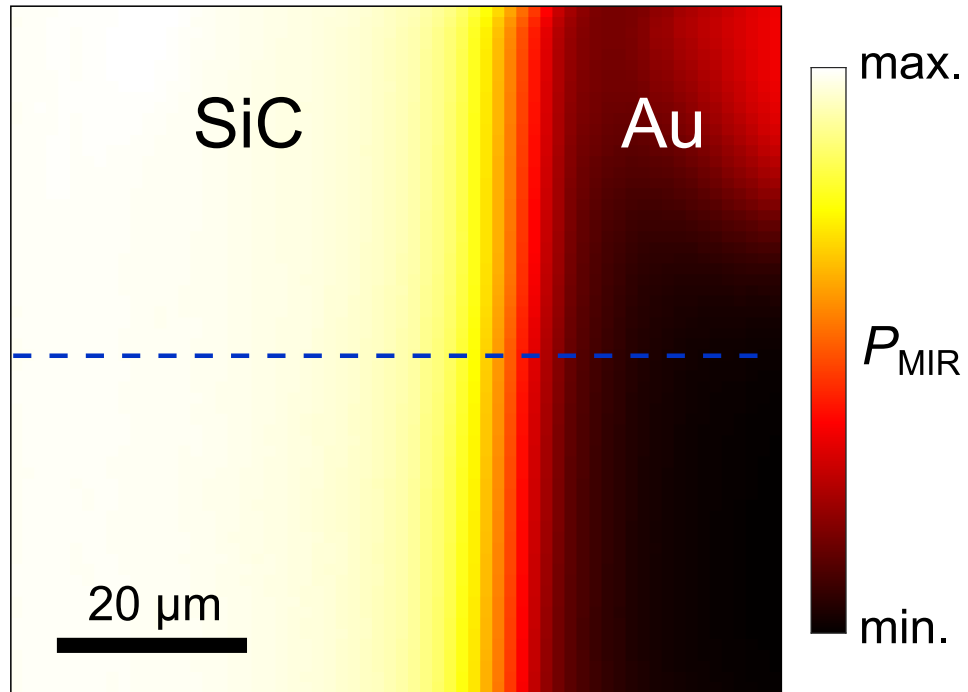**b**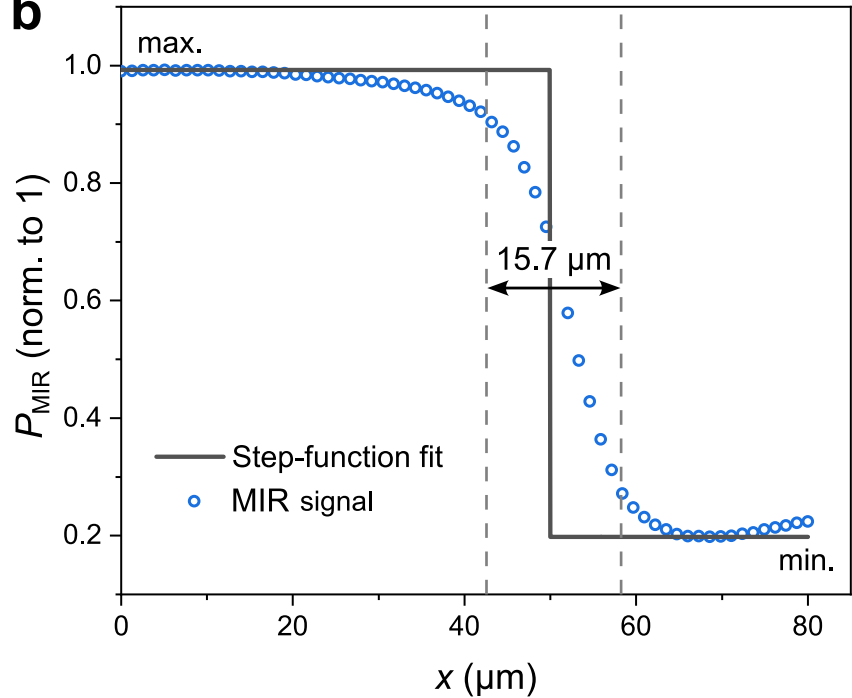

**a**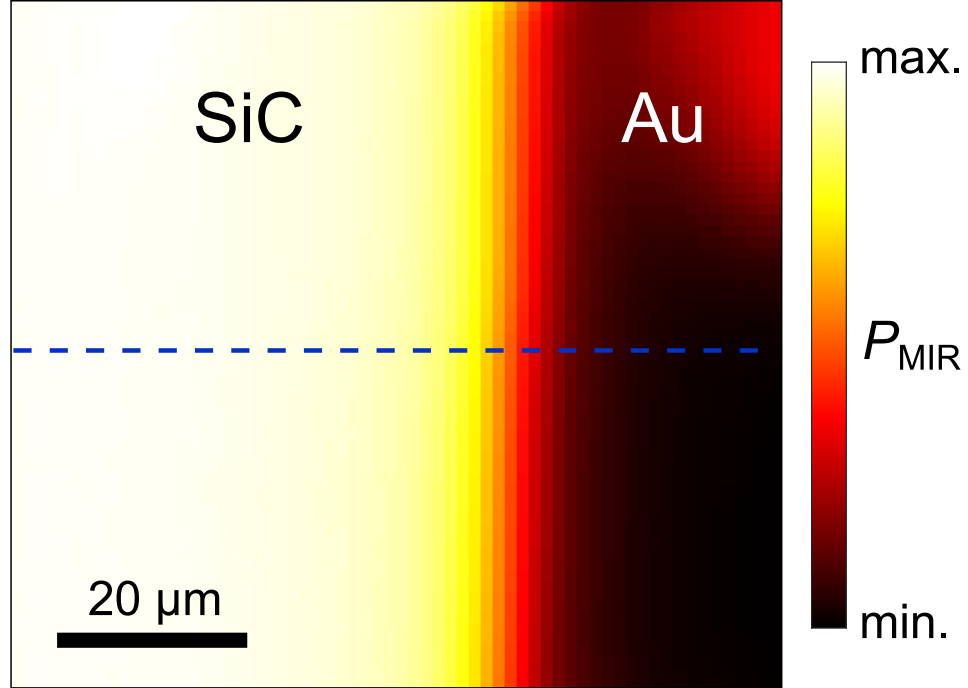**b**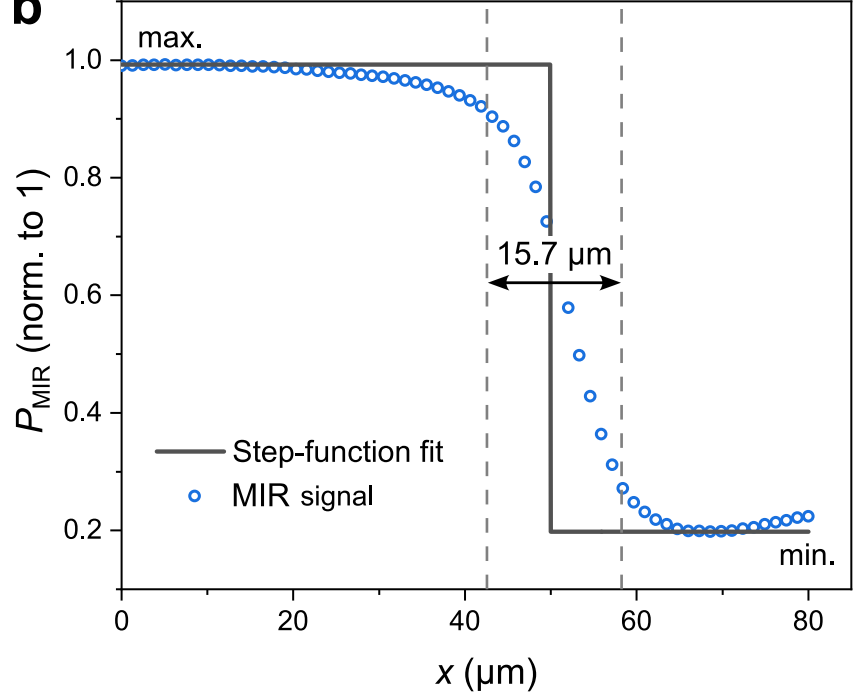

Supplement: Supplementary file 1 [file Au_SiC_res.pdf]
