# Supplementary material for: Electroluminescence and Energy Transfer Mediated by Hyperbolic Polaritons
Source: arXiv:2310.08351 source file (2024-12-02)

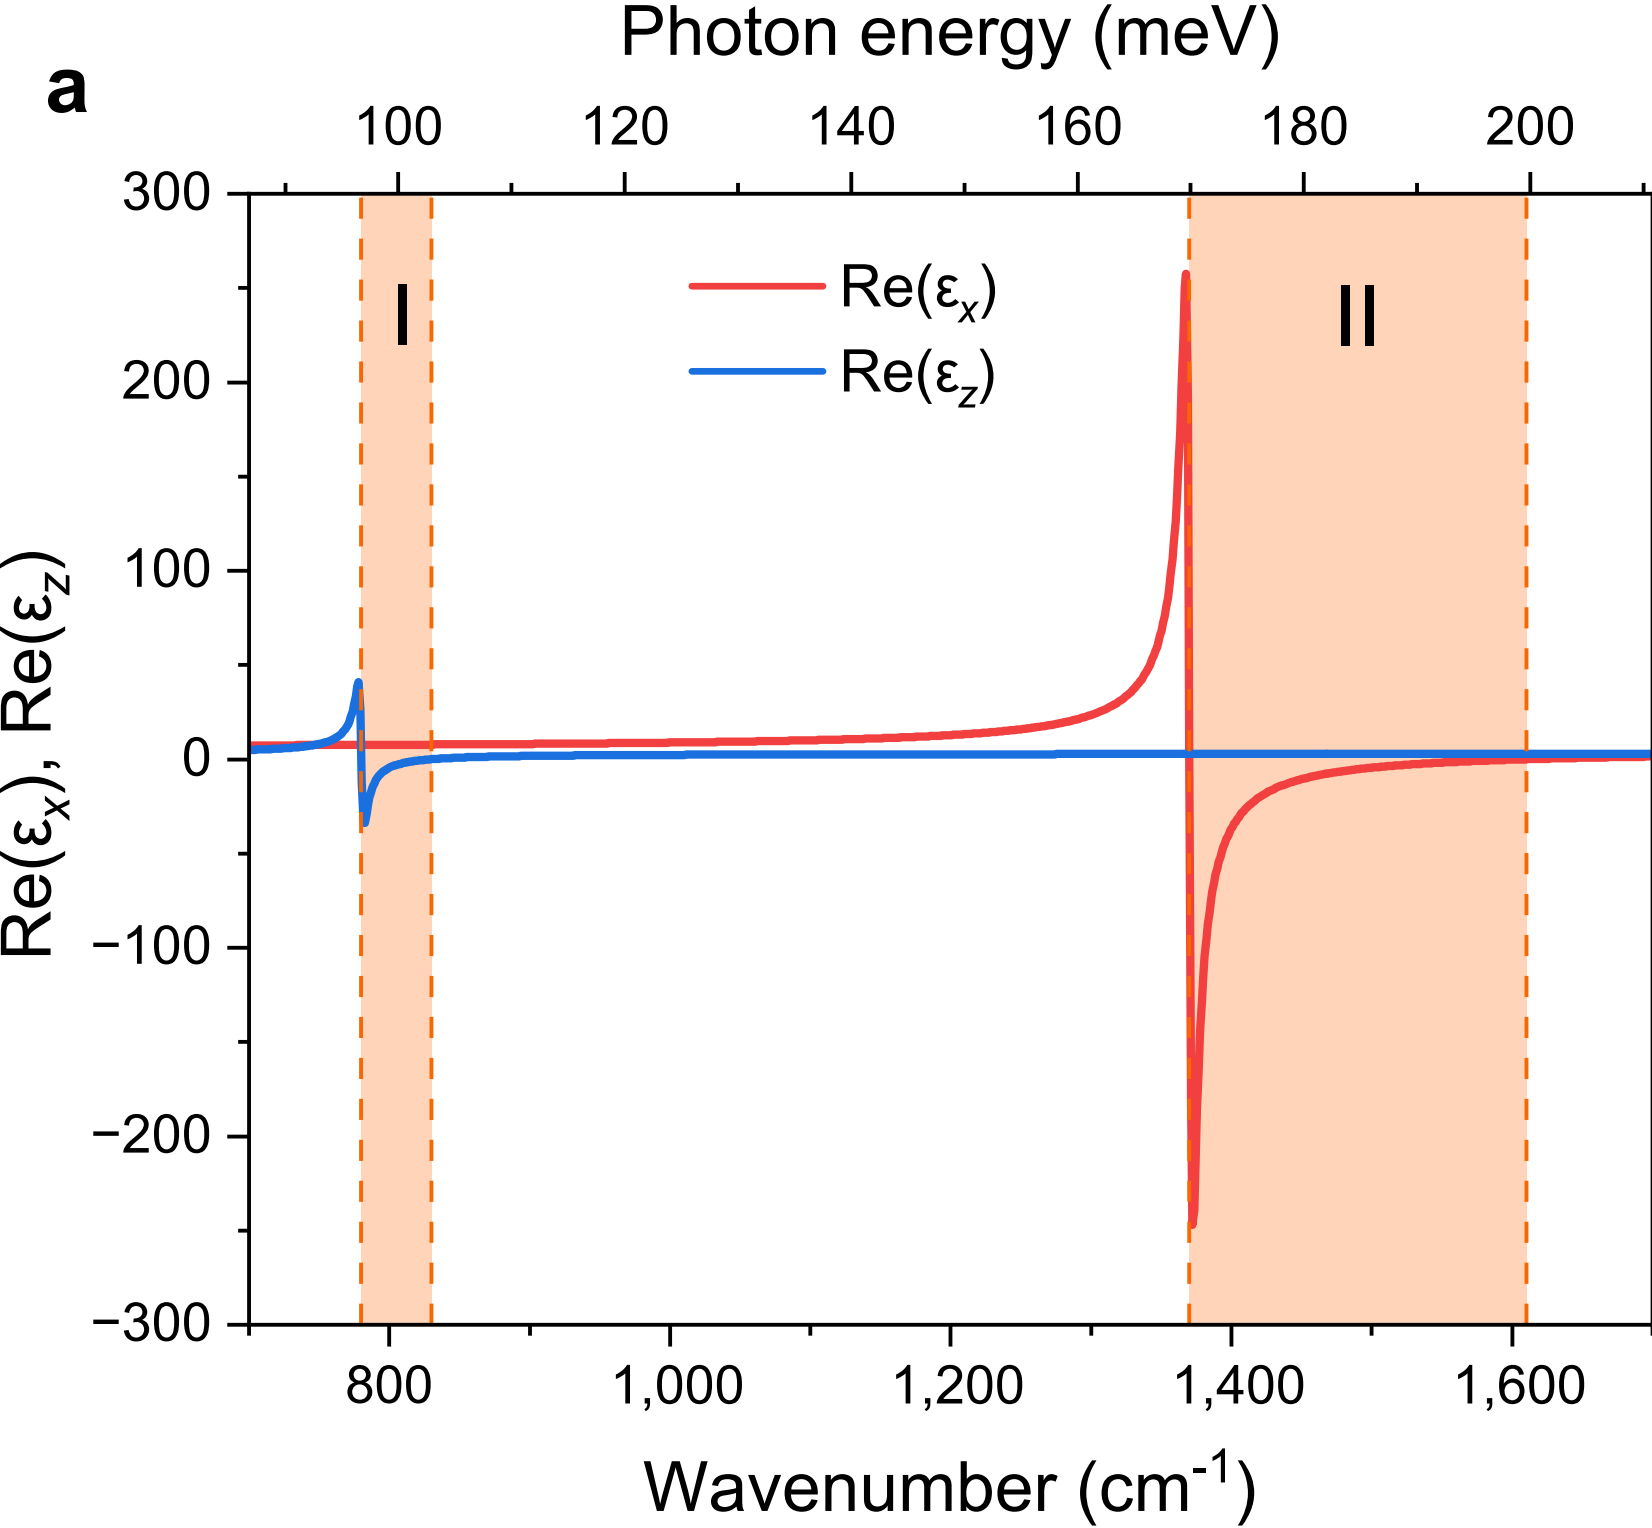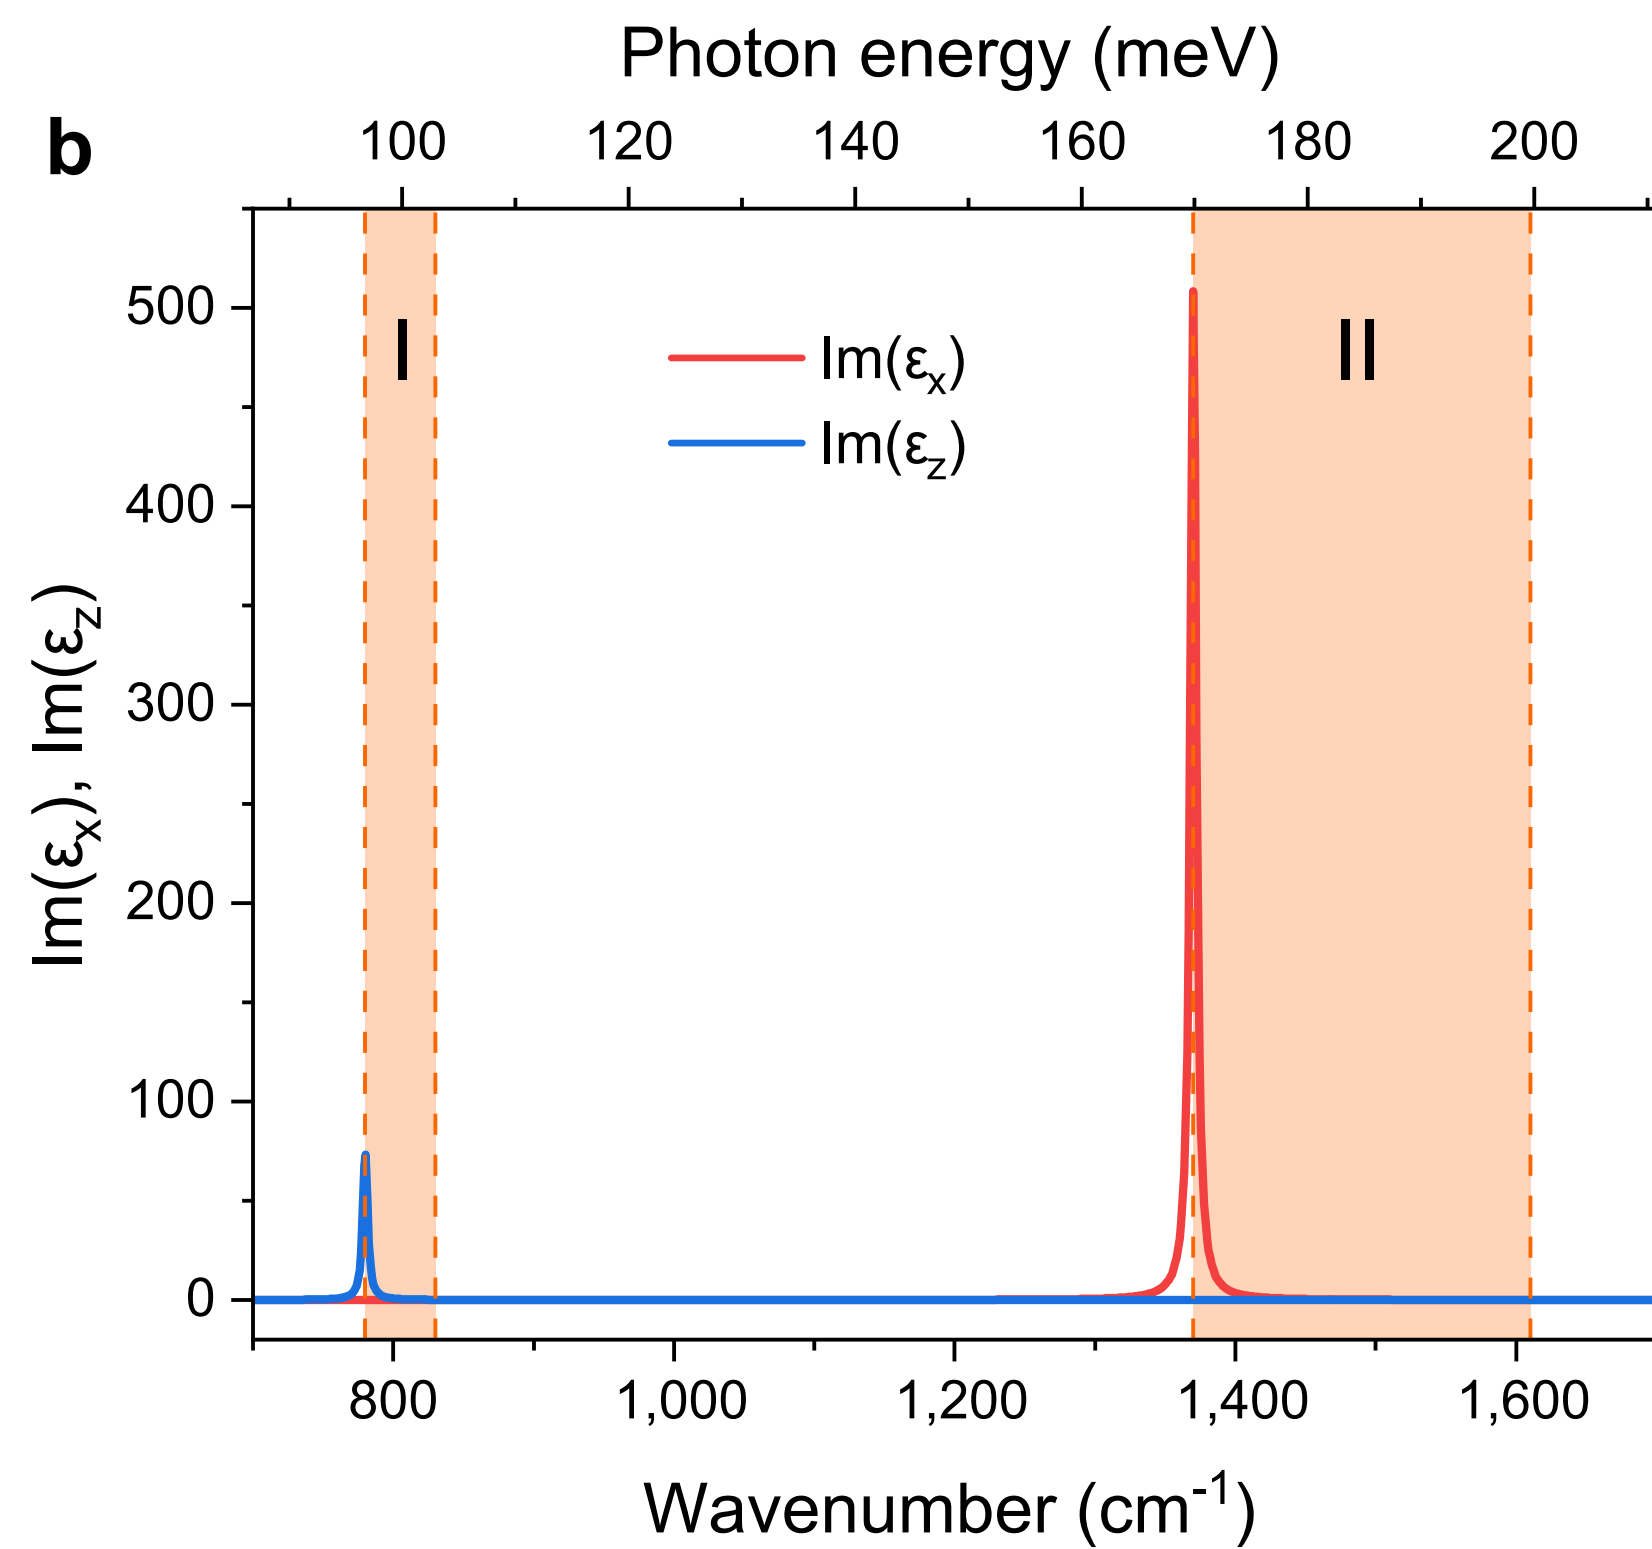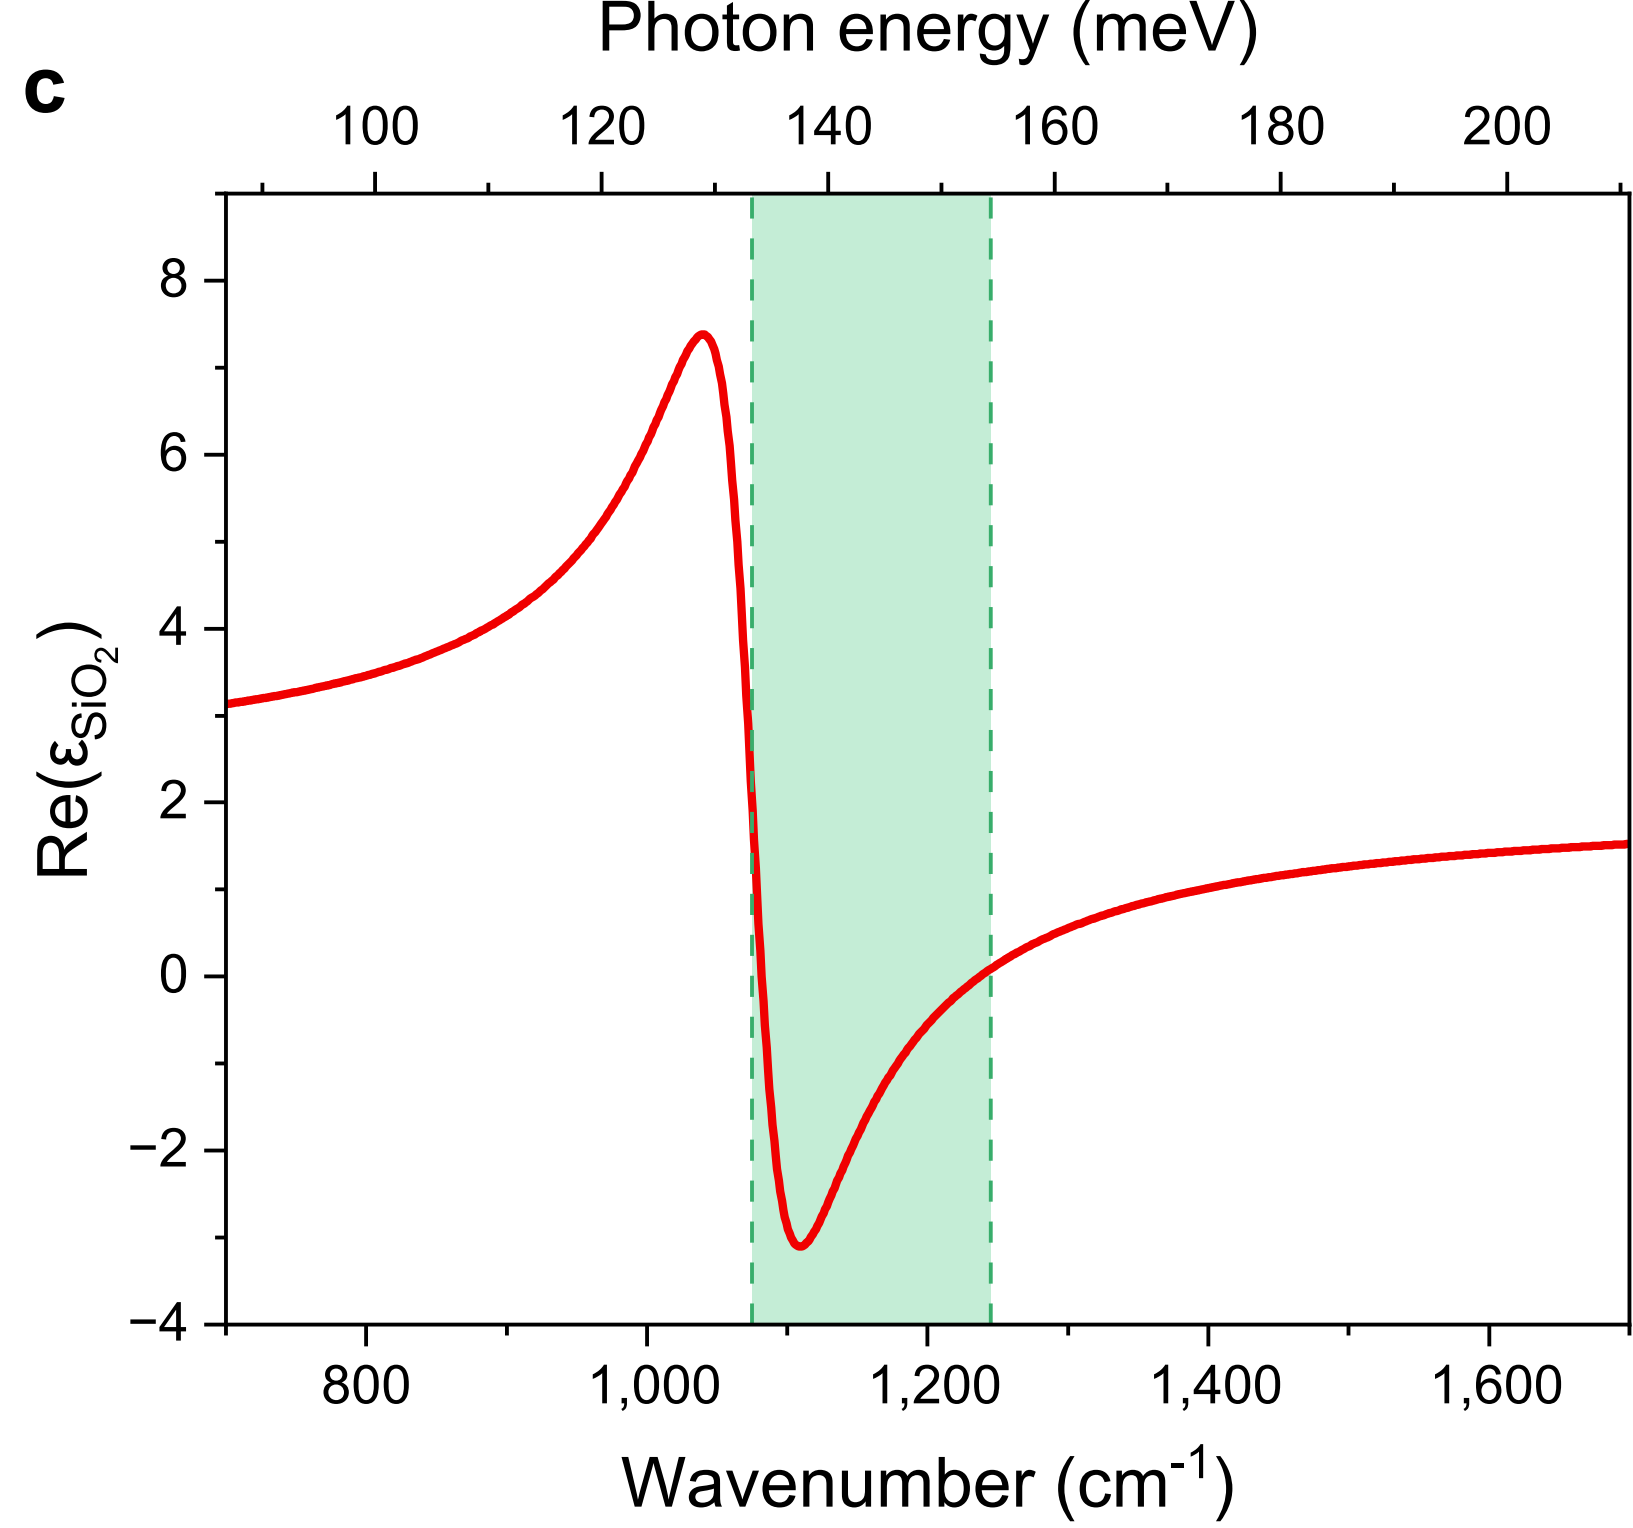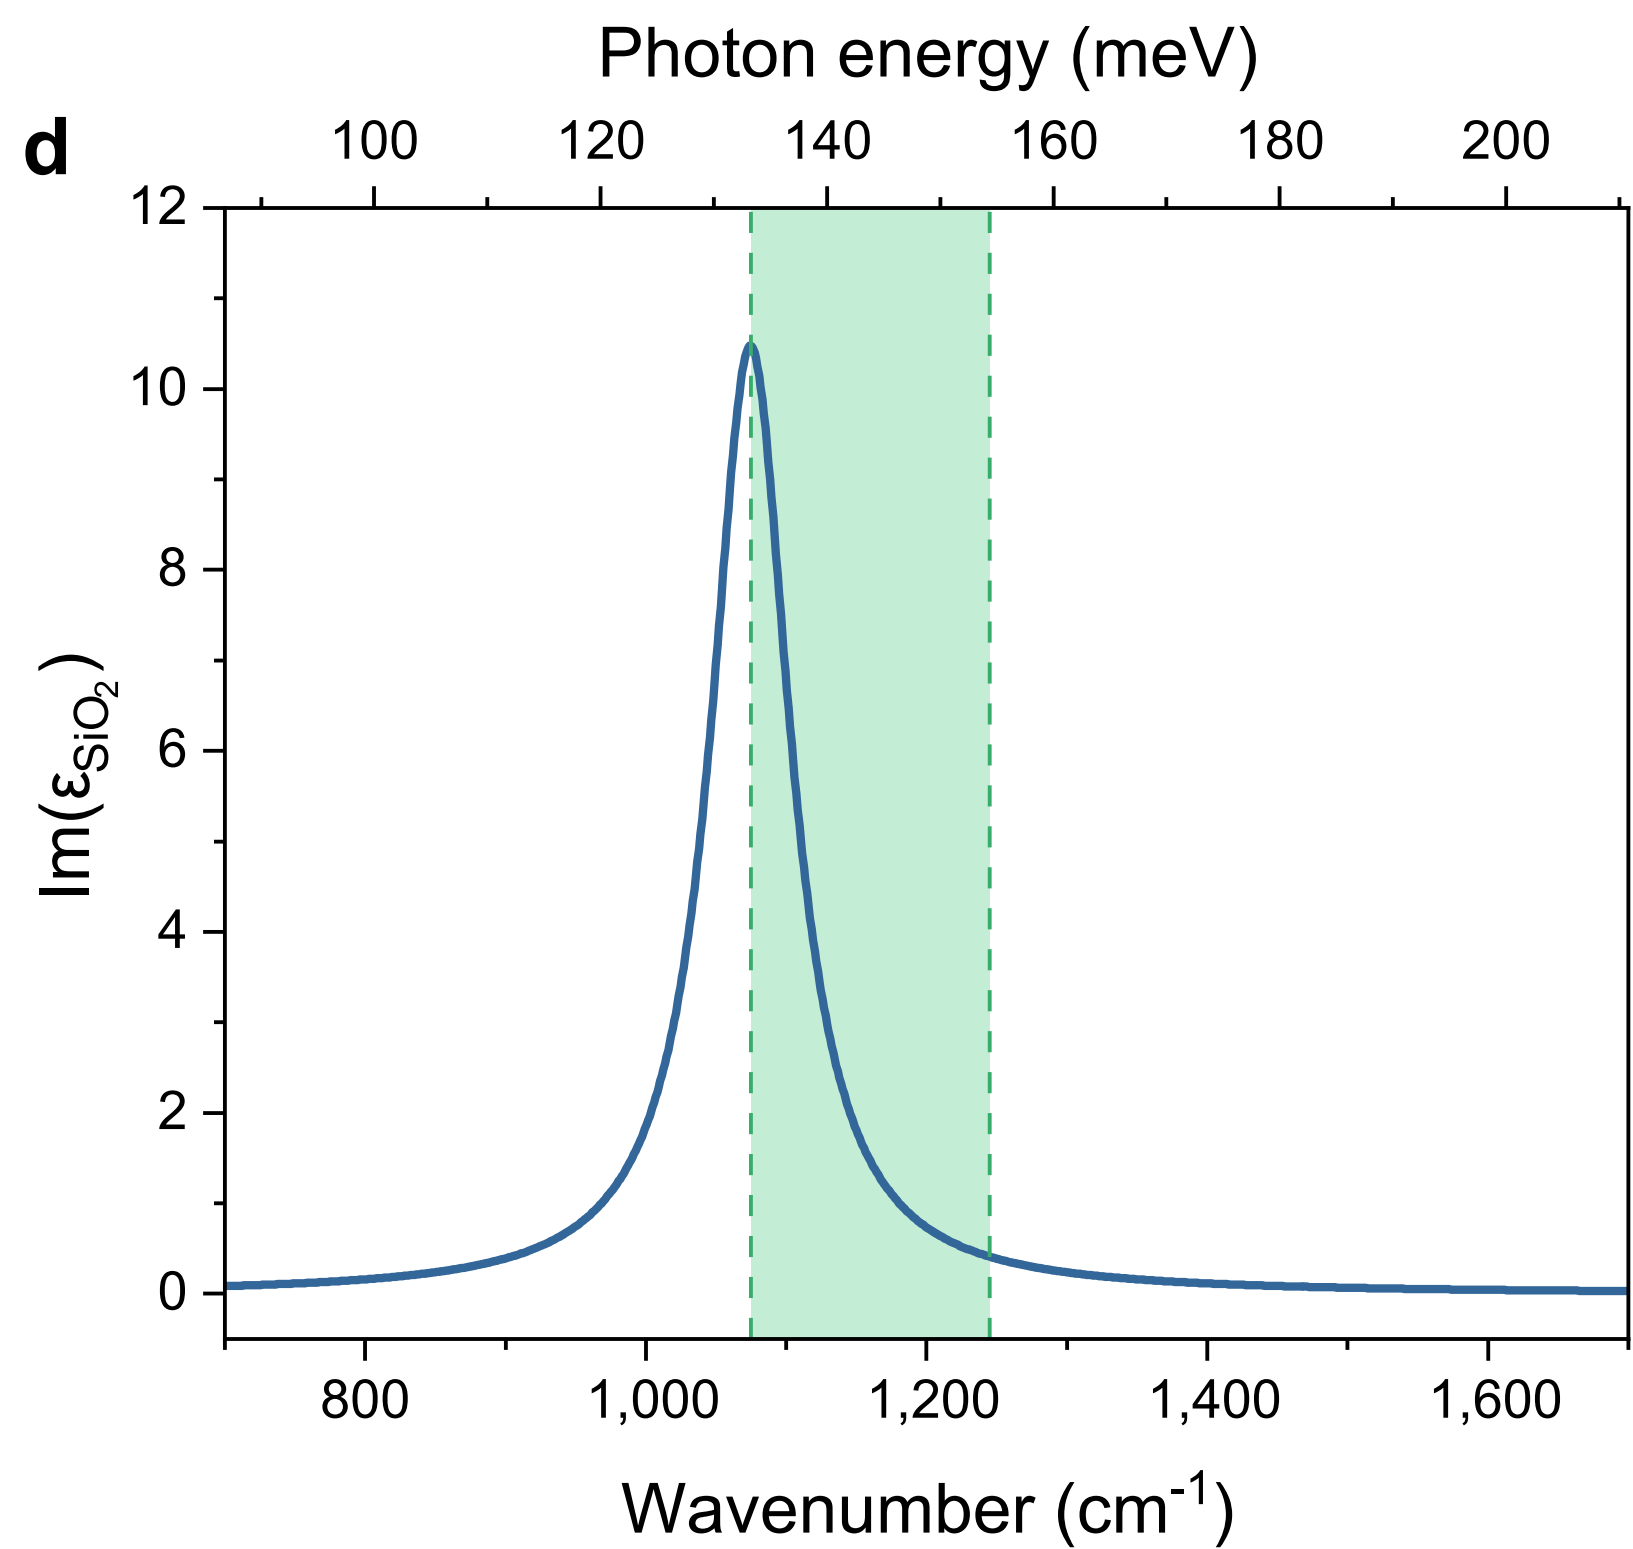

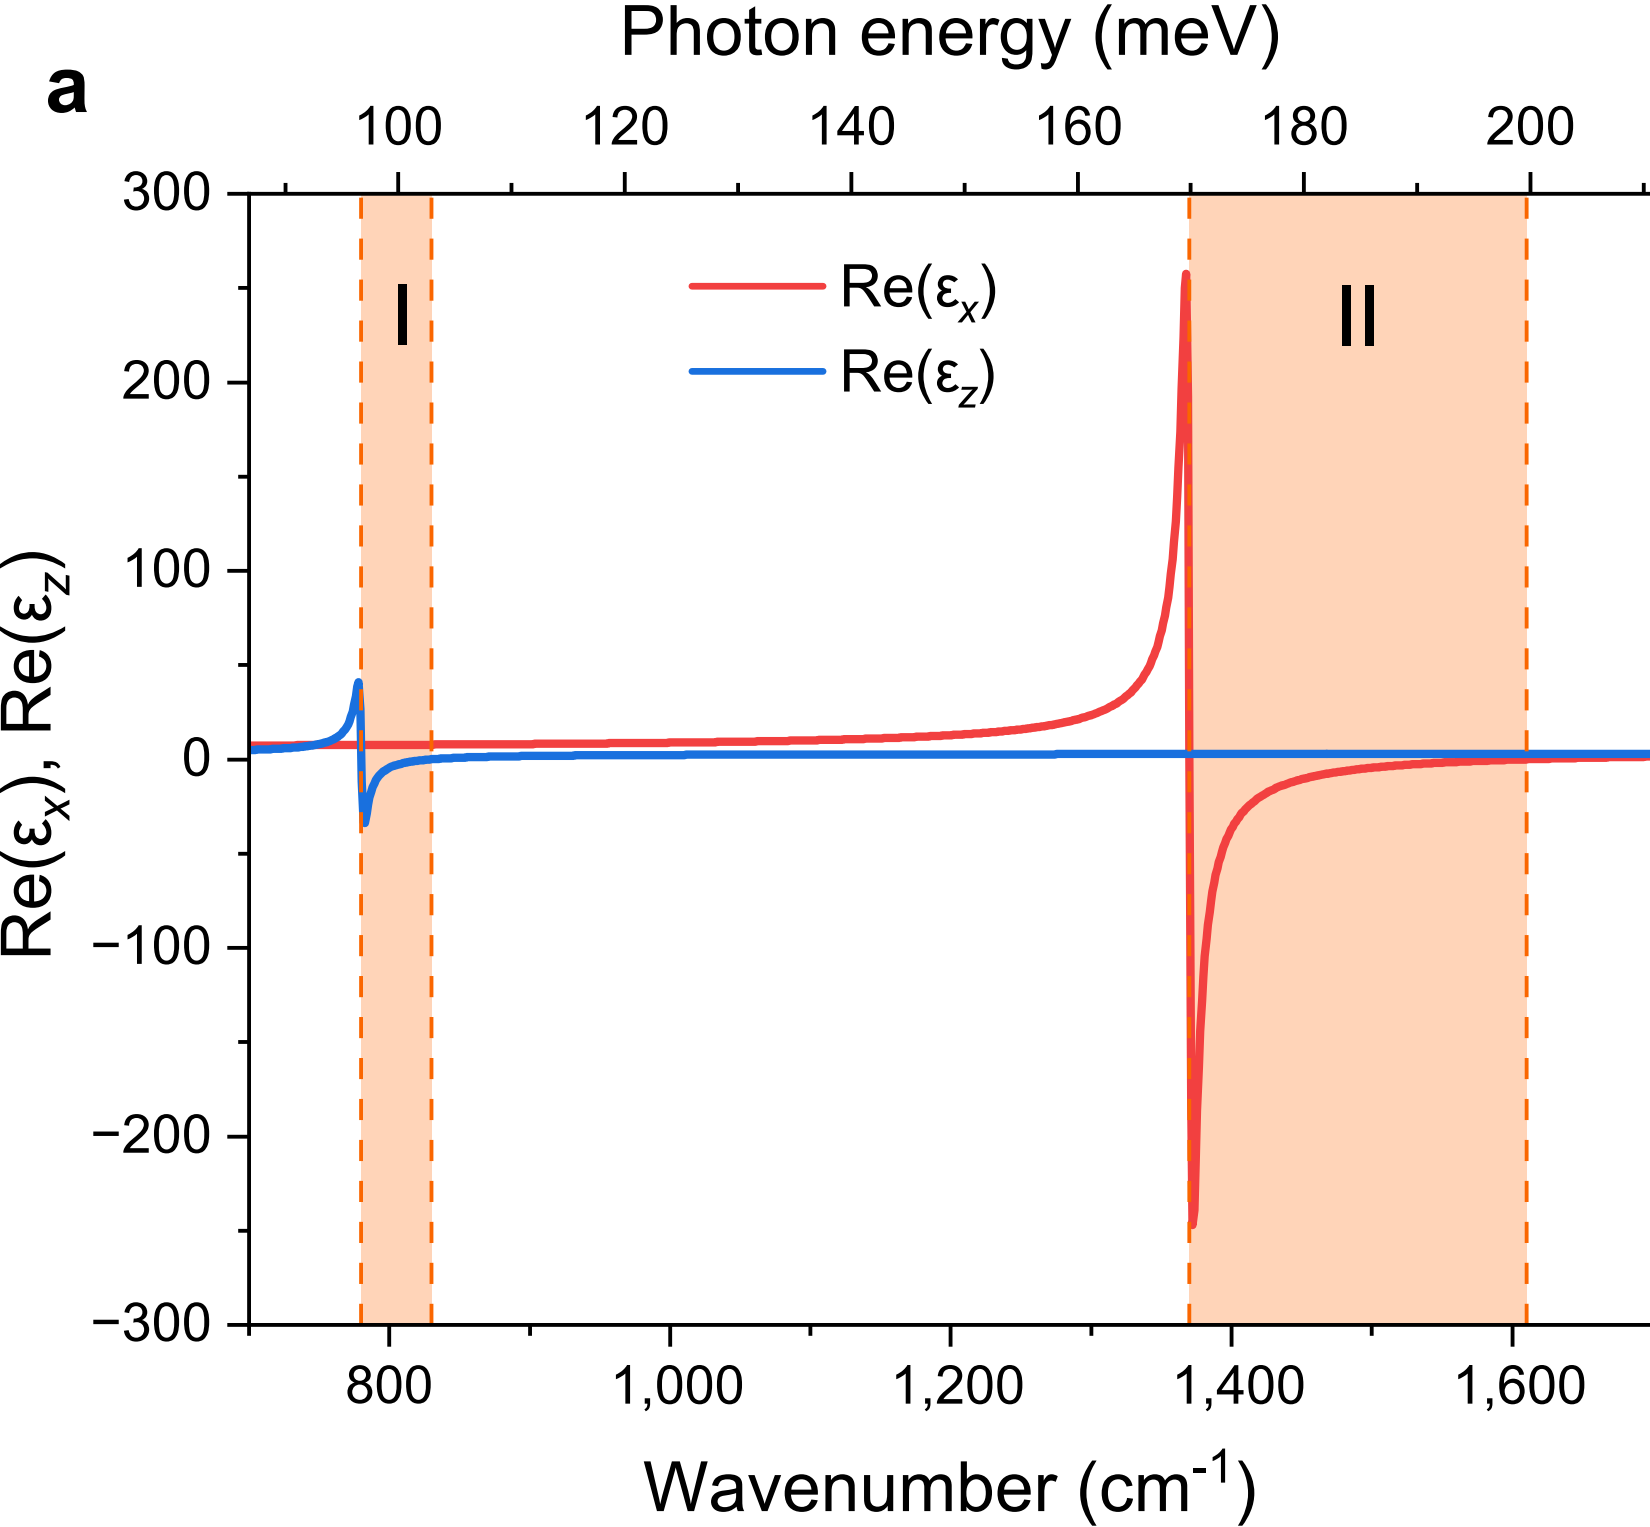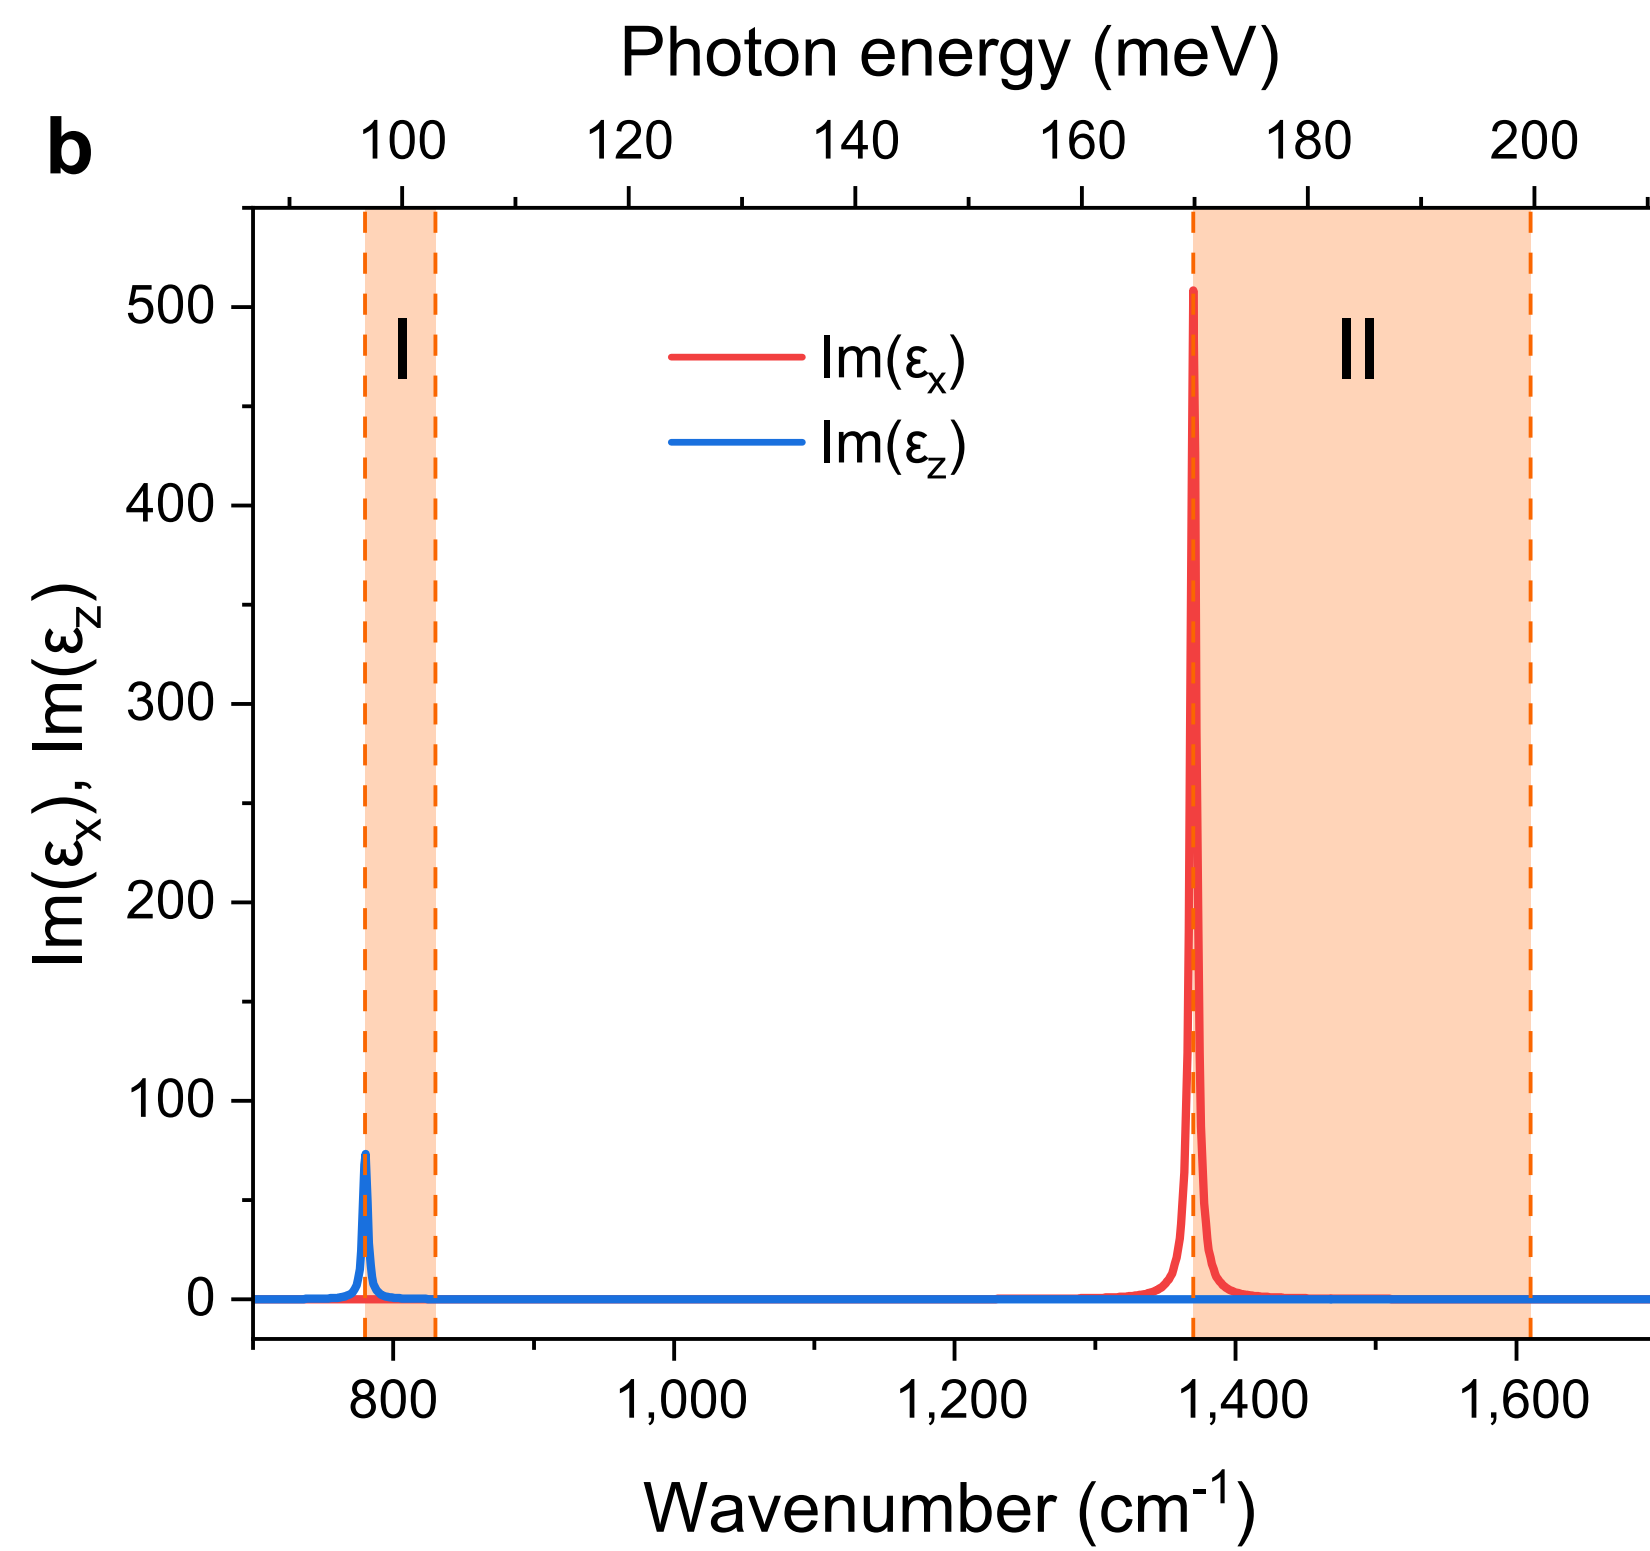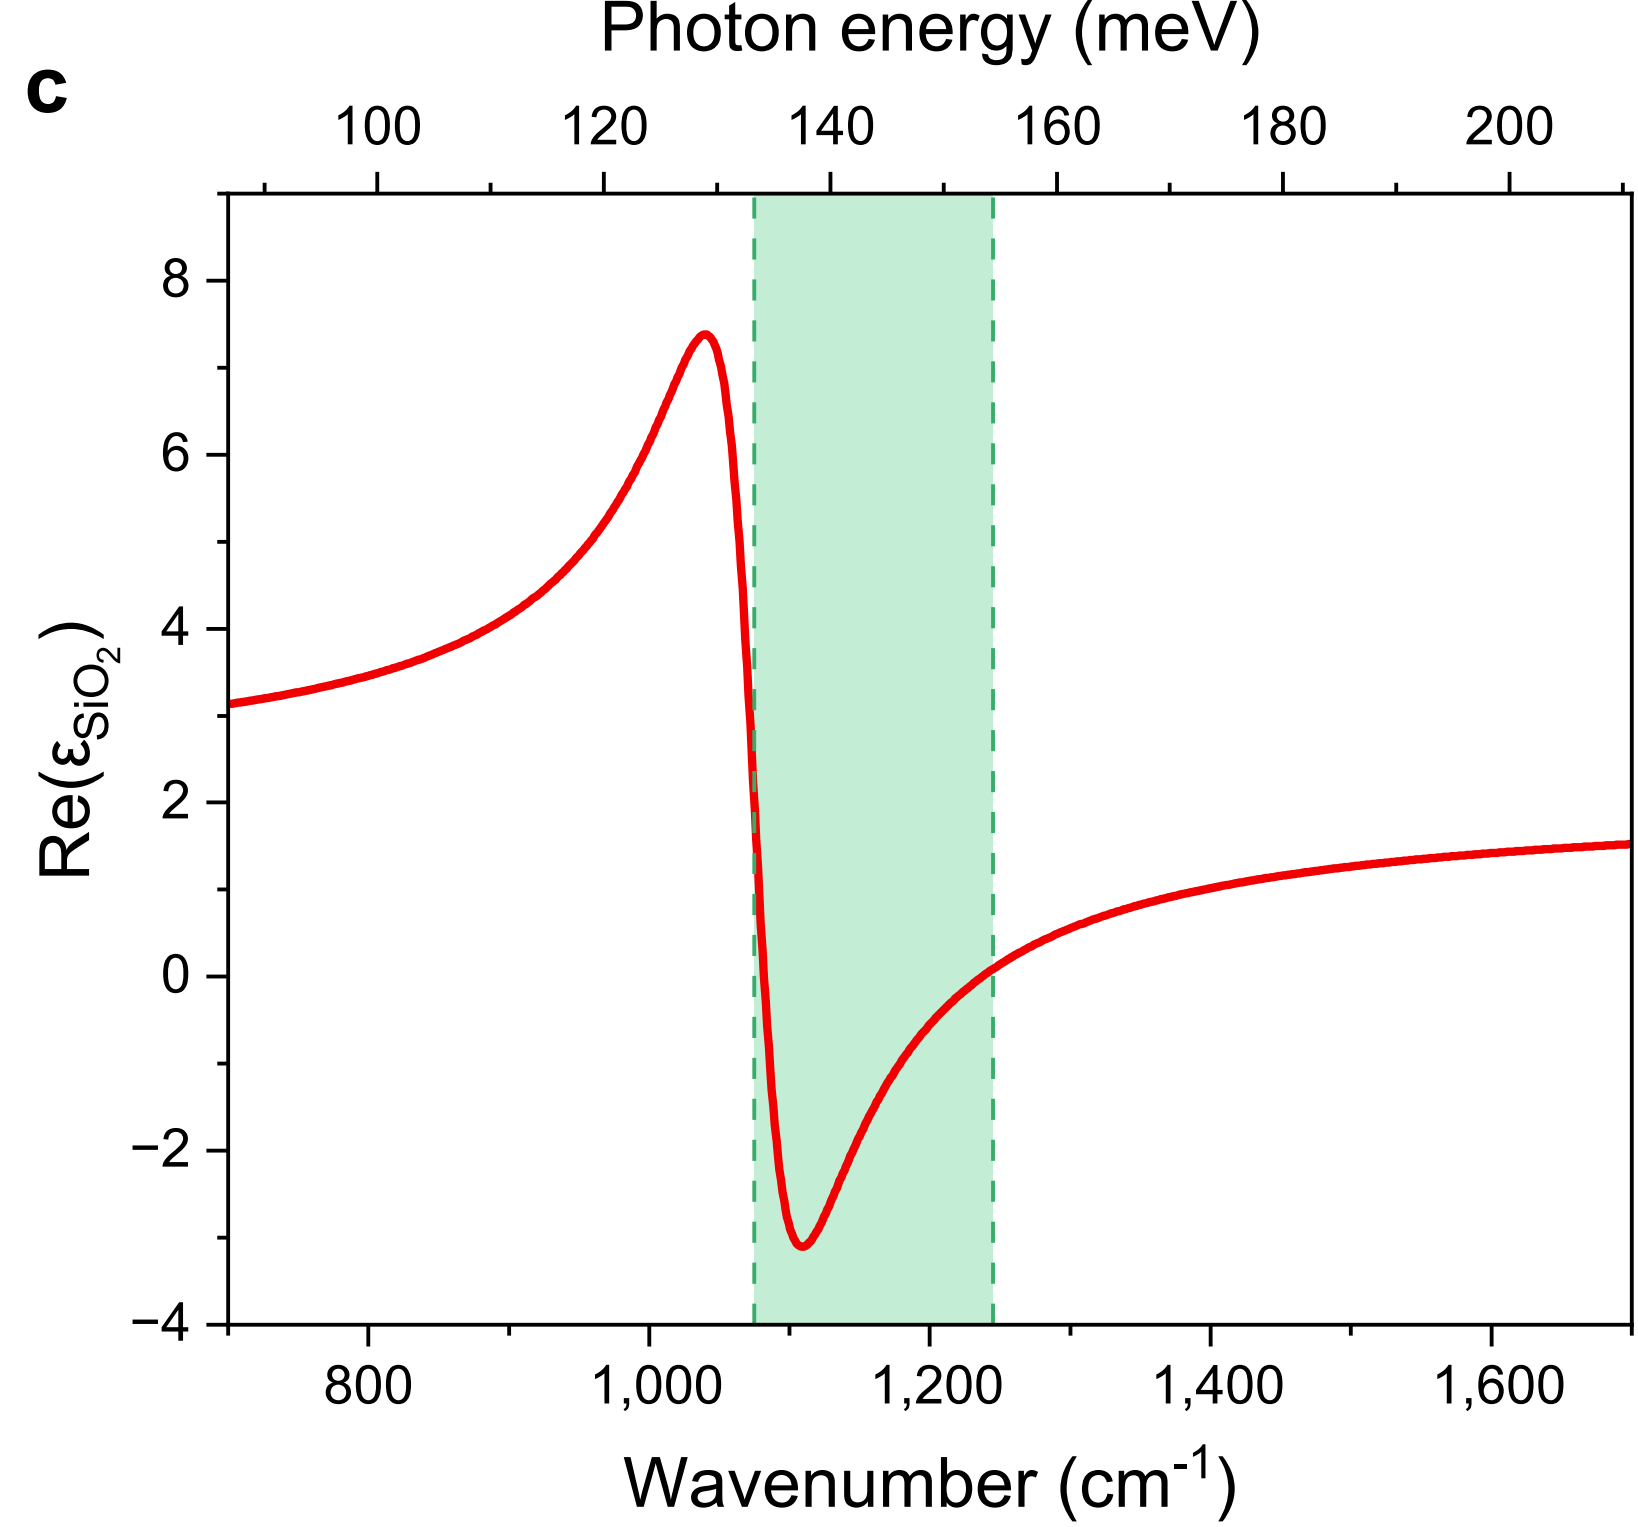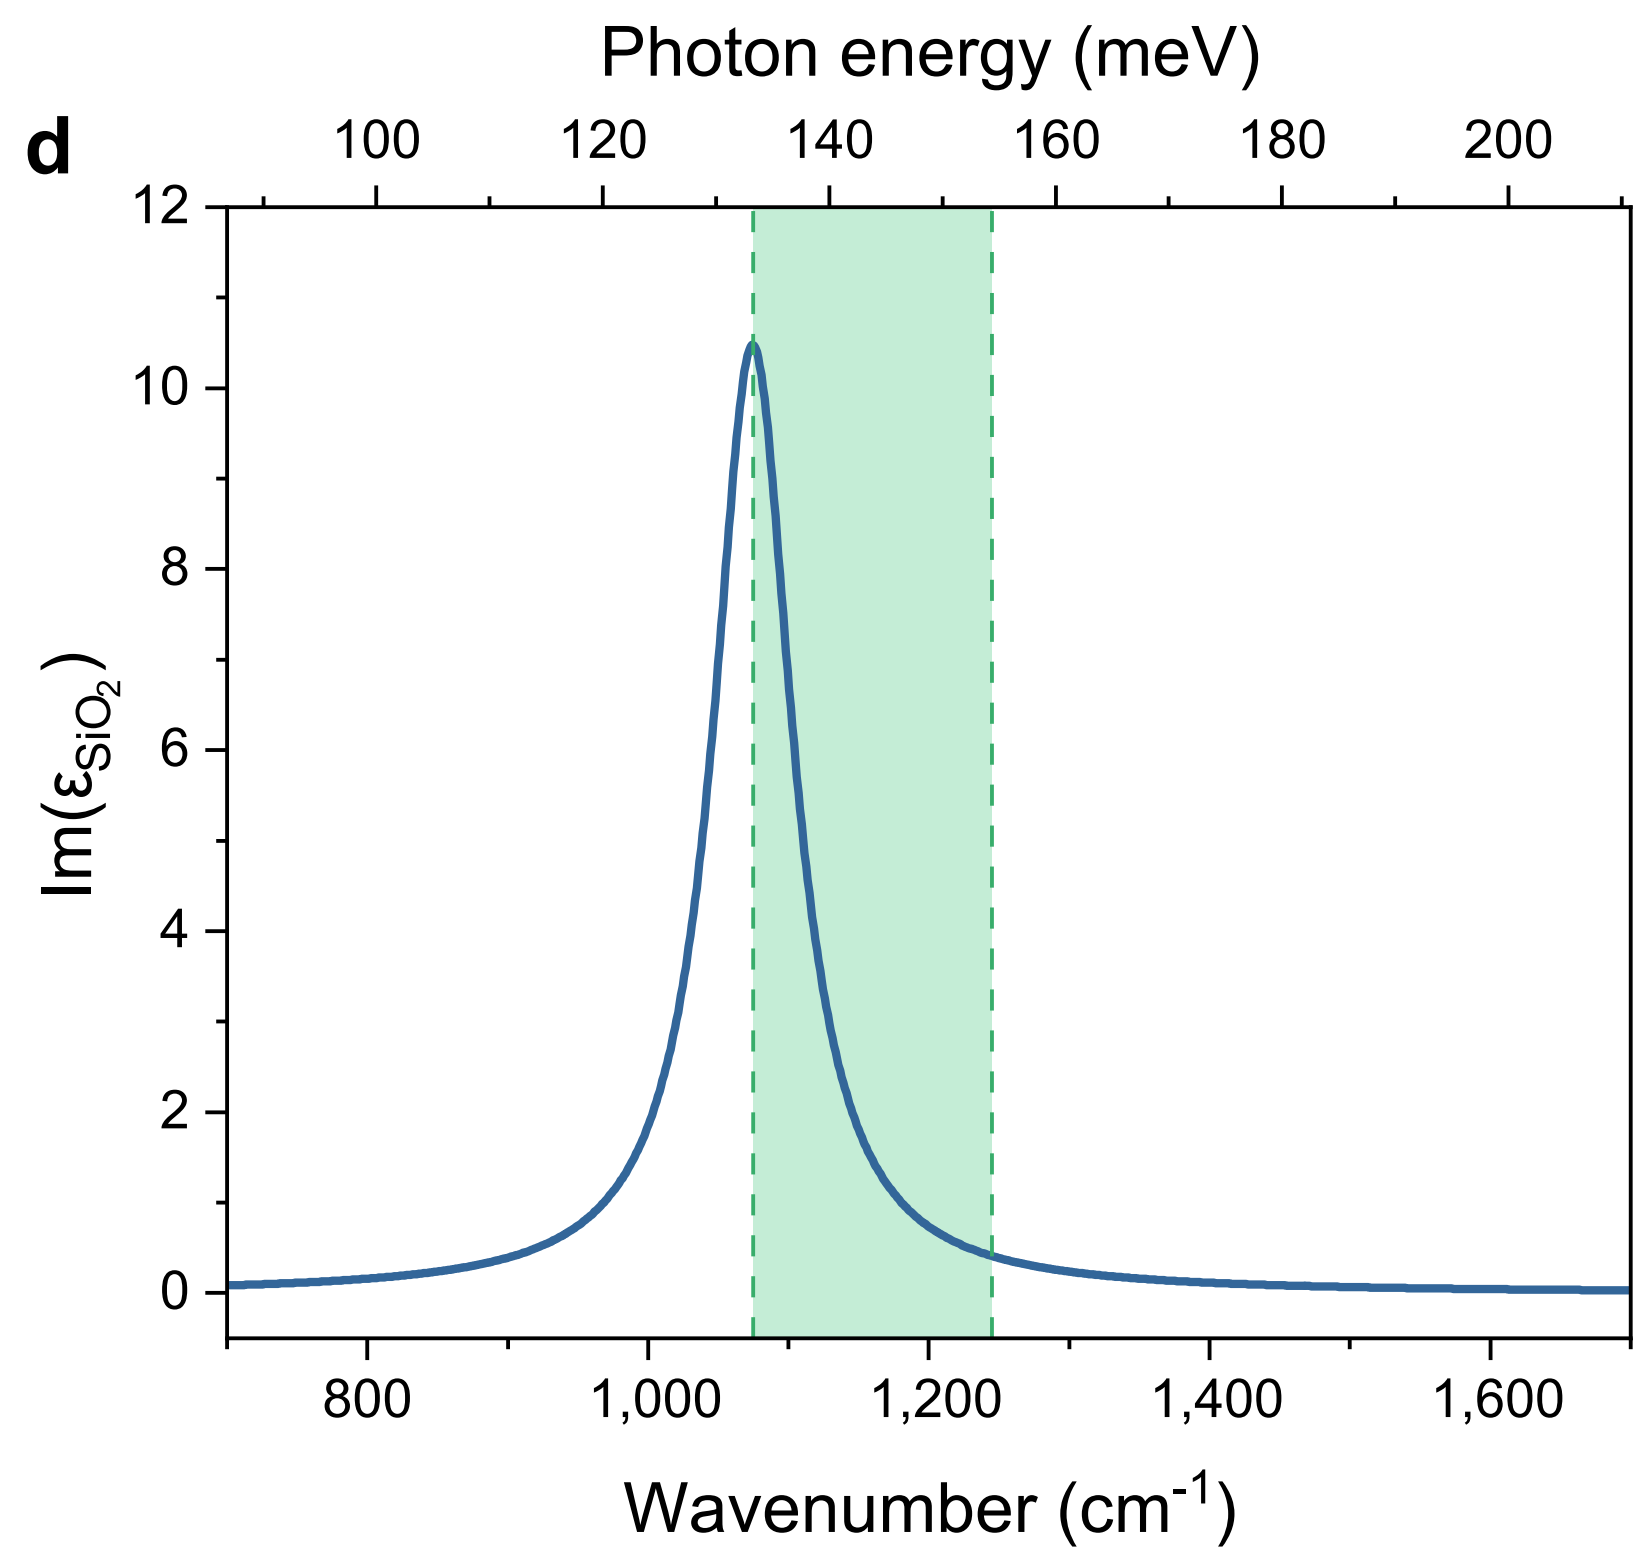

Supplement: Supplementary file 4 [file eps.pdf]
