# Supplementary material for: Electroluminescence and Energy Transfer Mediated by Hyperbolic Polaritons
Source: arXiv:2310.08351 source file (2024-12-02)

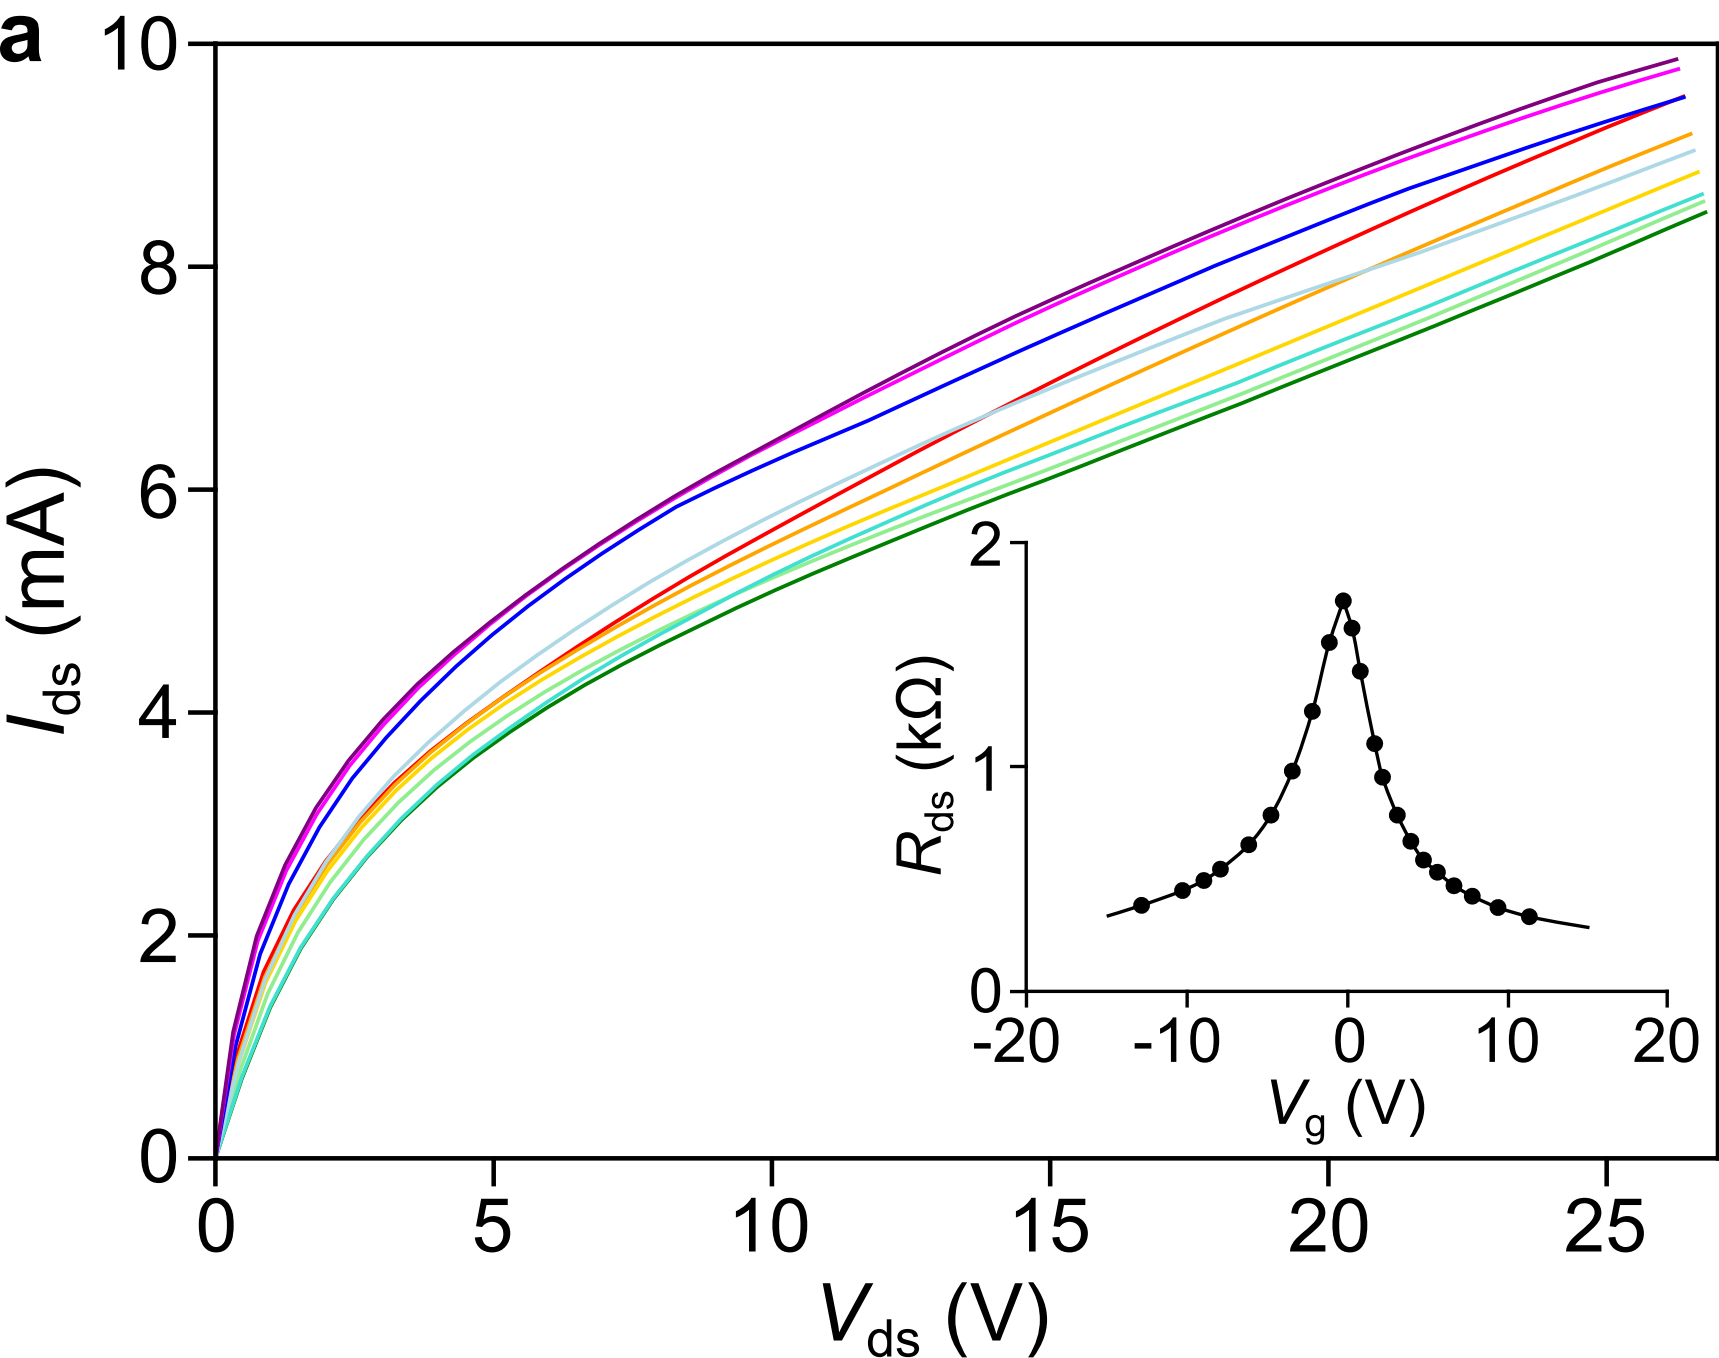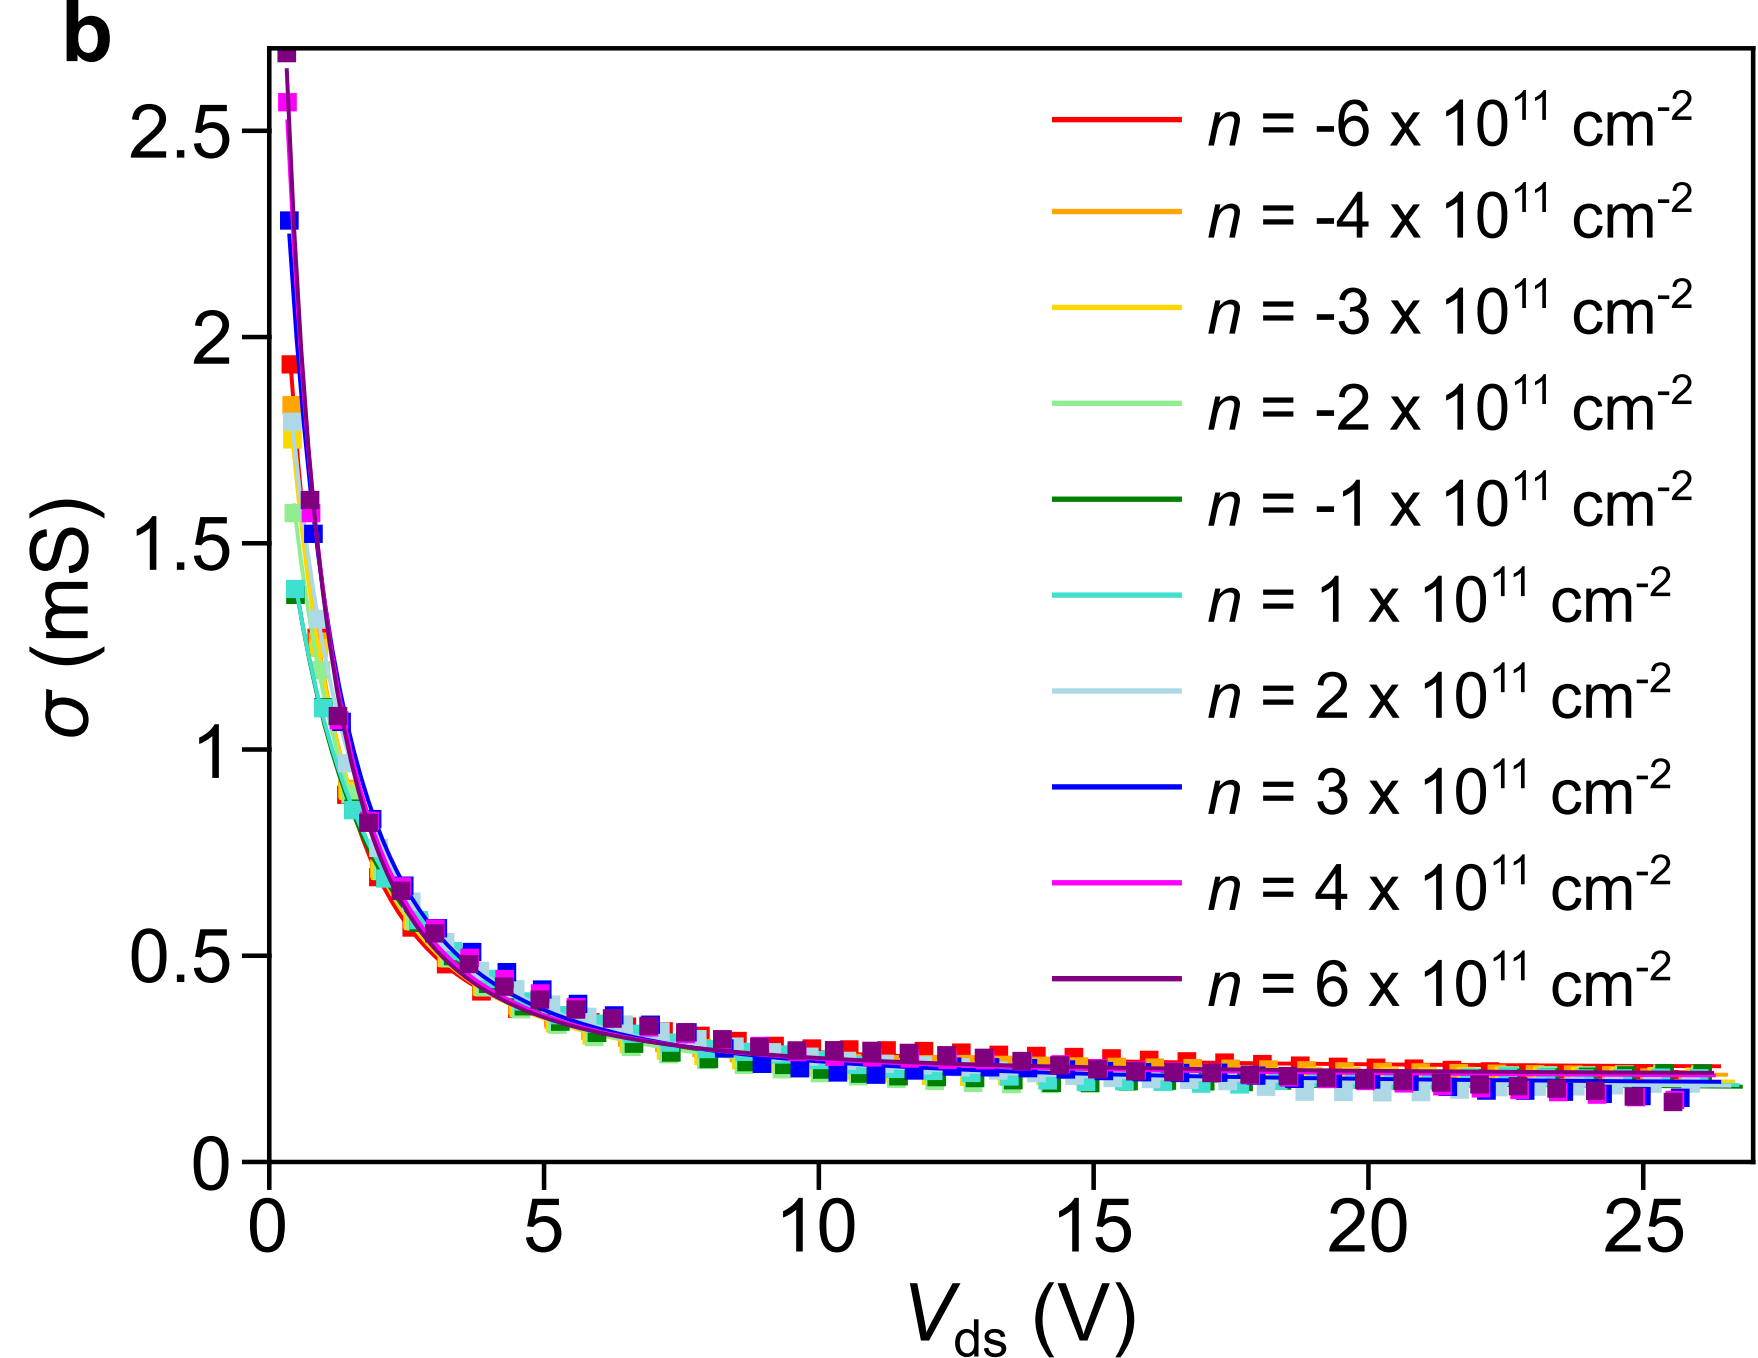

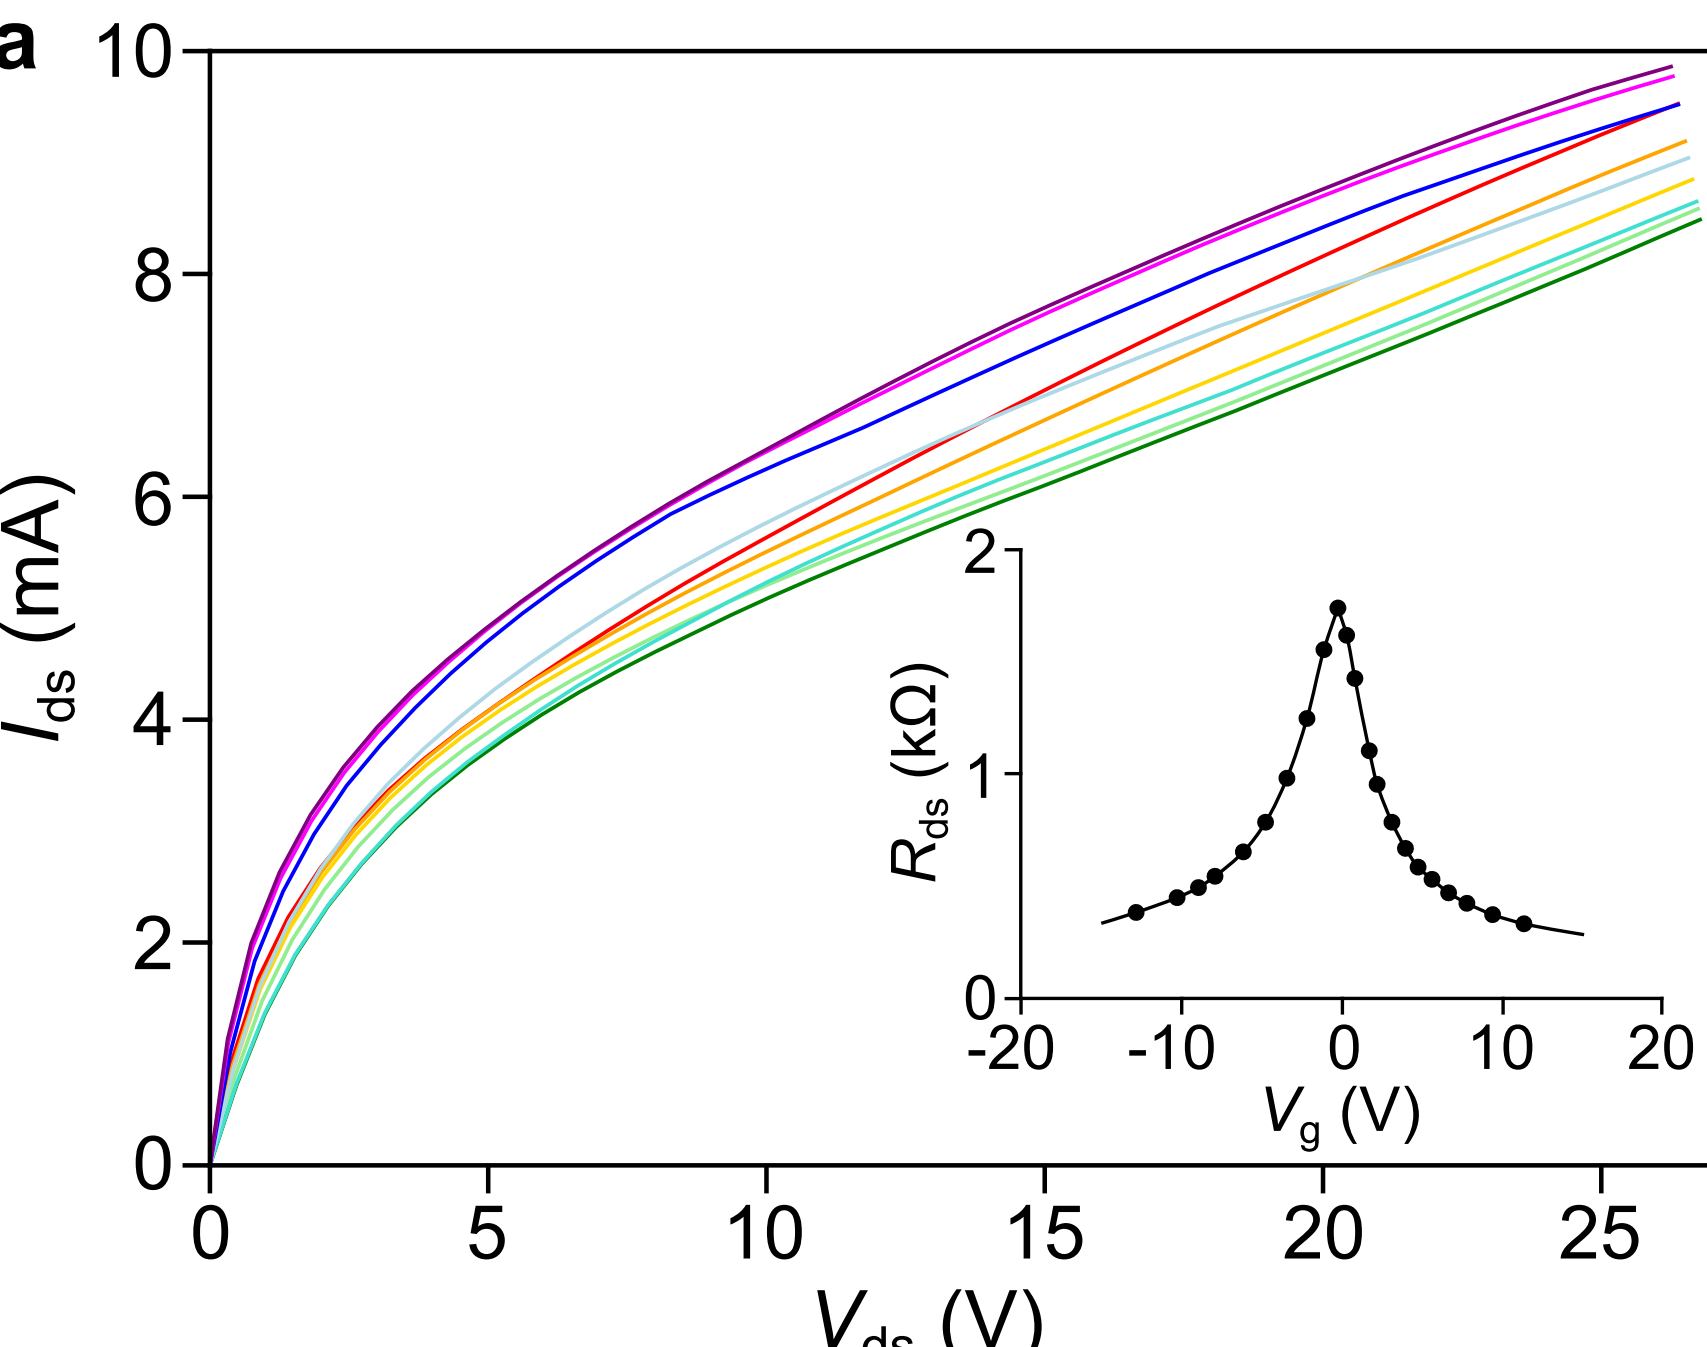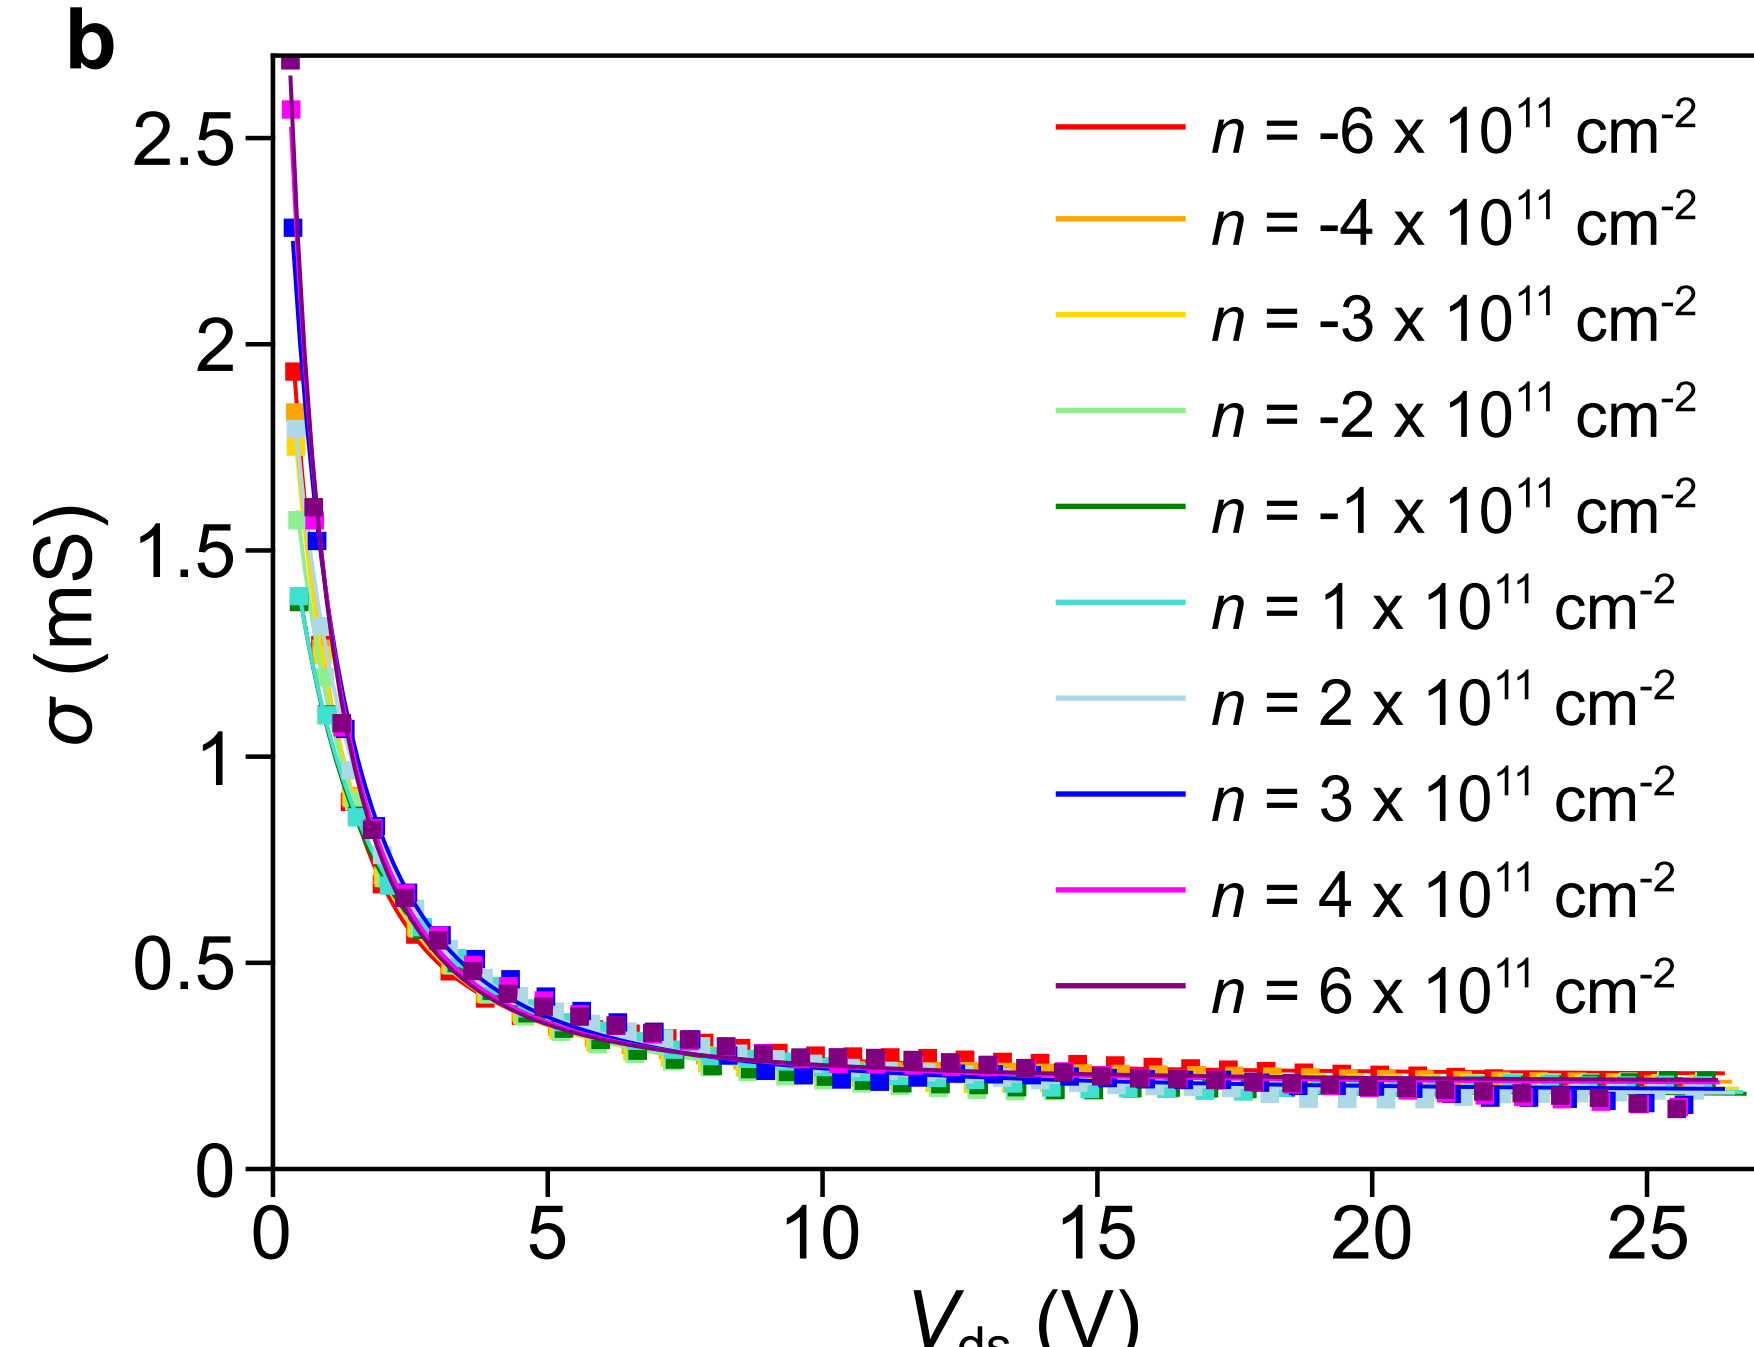

Supplement: Supplementary file 7 [file transport_TR2_v2.pdf]
